# Supplementary material for: Feasibility Study of LIMMS, A Multi-Agent Modular Robotic Delivery System with Various Locomotion and Manipulation Modes
Source: arXiv:2208.11252 source file (2022-08-24)
Supplement: Supplementary file 1 [file SA1_appendix.tex]

\section{Appendix}
\label{sec:appendix}

I am the appendix.
